# Supplementary material for: Asynchronous Federated Learning with Reduced Number of Rounds and with Differential Privacy from Less Aggregated Gaussian Noise
Source: arXiv:2007.09208 source file (2020-07-17)
Supplement: Supplementary file 2 [file 07_Appendix_FL.tex]

\section{Appendix Federated Learning}

\subsubsection{Categorization of Federated Learning}

\subsection{Categorization of Federated Learning}
In this section, we discuss how to categorize federated learning based on the distribution characteristics of the data \cite{yang2019federated,tianli2019federated}. The feature and sample space of the data on local clients or data owners may not be identical, and we classify federated learning into horizontally federated learning, vertically federated learning and federated transfer learning based on how data is distributed among clients in terms of the feature and sample space.

\textbf{Horizontal Federated Learning or sample-based federated learning} \cite{mcmahan,tianli2019hetero,keith,jakub,jakub2}, is applied in the scenarios that local data sets in clients share the same feature space but different in samples. A typical architecture for a horizontal federated learning system is shown in Figure $\ref{fig:horizon}$. In this system, $k$ clients with the same data structure collaboratively train independently global model with the help of a parameter server. In addition, a typical assumption \cite{phong} is that the participants are honest while the server is honest-but-curious, hence no leak information from any participants to other participants and the server is allowed.

\begin{figure}[!tbp]
  \centering
  \begin{minipage}[b]{0.45\textwidth}
 \includegraphics[width=\columnwidth]{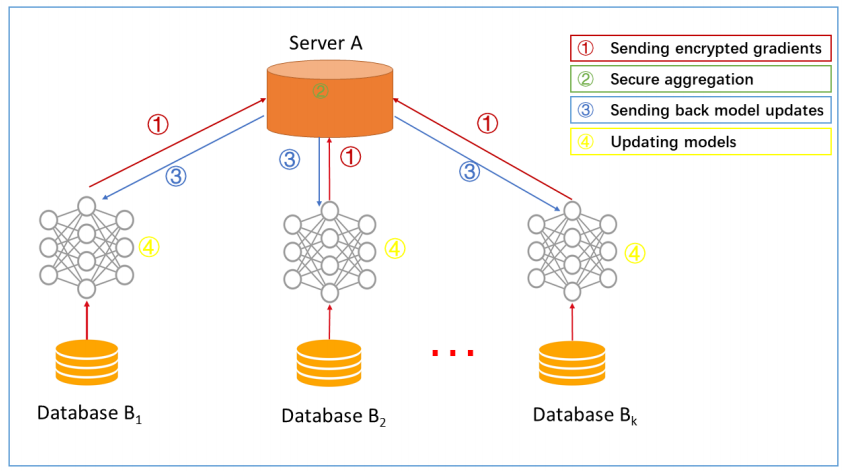}
    \caption{Architecture for a horizontal federated learning system \cite{yang2019federated}}
\label{fig:horizon}
  \end{minipage}
  \hfill
  \begin{minipage}[b]{0.5\textwidth}
  \includegraphics[width=\columnwidth]{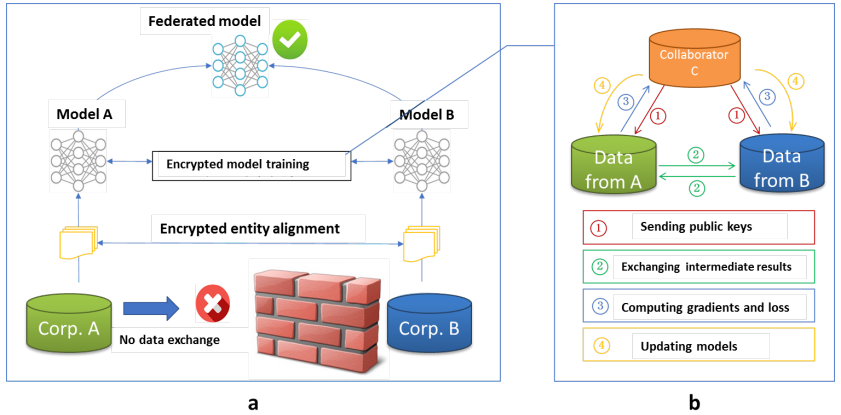}
    \caption{Architecture for a vertical federated learning system \cite{yang2019federated}}
    \label{fig:vertical}
  \end{minipage}
\end{figure}

% \begin{flushleft}
\textbf{Vertical federated learning or feature-based federated learning} \cite{richard,yang2019federated,hardy2017private} is applied in cases that data sets in client sides share the same sample space but differ in feature space (shown in Figure $\ref{fig:vertical}$a,b). It is the process of aggregating these different features and computing the training loss and gradients in a privacy-preserving manner to build a model with data from parties collaboratively. In addition, a vertical federated learning system typically assumes honest-but-curious participants. In the security perspective, it means that the adversary can only learn data from the corrupted clients but not data from other clients or from server. Recently, there are a lot of researches which have proved that FL can work very well with various machine learning models (for example, logistic regression, tree structure and neural network) \cite{gascon2016secure,karr2009privacy,vaidya2002privacy,wan2007privacy}.
% \end{flushleft}

% \begin{flushleft}
\textbf{Federated Transfer Learning} \cite{pan2009survey} can be used to the scenarios that the data sets in client sides are different from in both sample spaces and feature space, so transfer learning technique can handle the problem of lacking data (few samples and features) or weak supervision (few labels). We can distinguish the major difference between vertical FL and federated transfer learning is that federated transfer learning can exchange models among clients, which is not seen in vertical FL (shown in figure $\ref{fig:vertical}$a,b). However, the set of overlapped data from clients could be small (for example the different businesses in reality) and make federated transfer learning less attractive and effective. Interestingly, the paper in \cite{yang2018secureftl} proposes a possible solution to these above challenges by exchanging the models using homomorphic encryption among clients, which leverages the transfer learning technique proposed by \cite{pan2009survey} to provide solution for training FL with the sample and feature space under a data federation and privacy-preserving constraints.

\subsubsection{Notes on Asynchronous federated optimization algorithm}
Asynchronous training technique \cite{zinkevich,lian,zheng,meng2017asynchronous,shi2019distributed} is widely used in traditional distributed stochastic gradient descent (SGD). Typically, asynchronous SGD converges faster than synchronous SGD. However, classic asynchronous SGD directly sends gradients to the server after each local update, which is not practical for edge devices (such as mobile or IoT devices) due to the unreliable and slow communication.

The paper in \cite{cong,yang} proposed asynchronous training, and combine it with federated optimization. Specifically, the server and workers conduct updates asynchronously: the server immediately updates the global model whenever it receives a local model from clients. Therefore, the communication between the server and workers is non-blocking and more effective. However, asynchronous FL can come without convergence guarantees and can diverge in practical settings when data are heterogeneous \cite{tianli2019federated}. Moreover, a temporally weighted aggregation strategy \cite{yang} is introduced on the server to make use of the previously trained local models and eventually enhances the accuracy and convergence of the central mode.

In addition to the performance and convergence guarantee of the federated system, we need to pay attention to what type of federated learning application having the potential to deploy in reality or industry. For example, a new asynchronous federated learning \cite{capota} is proposed to be used in reality, especially tack the challenging geospatial application: image classification based on geolocation using a state-of-the-art convolutional neural network.
